# Supplementary material for: Equilibrium Analysis of Customer Attraction Games
Source: arXiv:2307.07174 source file (2024-10-10)
Supplement: Supplementary file 1 [file appendix.tex]

%\section*{Appendix}

%\input{Source/Sequential}

\section{The Missing Proofs in Section \ref{Sec:basic}}

\section{Missing Proofs in Section \ref{Sec:asymmetric}}
